# Supplementary material for: Musicological, computational and conceptual aspects of first-species counterpoint theory
Source: arXiv:2102.11767 source file (2021-02-23)
Supplement: Supplementary file 1 [file supplement.pdf]

*Journal of Mathematics and Music*, **INSERT YEAR NONBOLD**
Vol. **INSERT NONBOLD**, No. **INSERT NONBOLD KEEP COMMA**, INSERT DOI LINK FROM PUBL

# Online Supplement to "Musicological, computational, and conceptual aspects of first-species counterpoint theory"

Juan Sebastián Arias-Valero[a*], Octavio Alberto Agustín-Aquino[b**], and Emilio Lluis-Puebla[a***]

[a]*Departamento de Matemáticas, Universidad Nacional Autónoma de México, Ciudad de México, México;*
[b]*Instituto de Física y Matemáticas, Universidad Tecnológica de la Mixteca, Huajuapan de León, México*

We reproduce the Python codes used in the main paper.

**Keywords:** Python

## Code 1. Strict style modulo translation

```
# PROGRESSIONS in a diatonic scale

# consonances

 # up to the tenth
Kt={0,3,4,7,8,9,12,15,16}

 # reduced
K={0,3,4,7,8,9}

# range of the voices in the diatonic scale

 # range cf start
X={0,2,4,5,7,9,11}
 # range dc start (plus up to a tenth from cf start)
rdc=X.union({12,14,16,17,19,21,23,24,26})

 # range cf end (plus up to the octave from cf start)
X1=X.union({x-12 for x in X},{x+12 for x in X})
 # range dc end (plus up to a tenth from cf end)
rdc1=X1.union({24,26,28,29,31,33,35,36,38})
```

* Email: jsariasv1@gmail.com
** Email: octavioalberto@mixteco.utm.mx
*** Email: lluisp@unam.mx

```
# counterpoint consonances

 # start interval
Cc={(x,k) for x in X for k in Kt if x+k in rdc}

 # end interval
Cc1={(x,k) for x in X1 for k in Kt if x+k in rdc1}

# possible progressions

P=set()
for i in Cc:
    for j in Cc1:
        # we only allow skips up to the octave in each voice
        x=j[0]-i[0]
        y=j[0]+j[1]-(i[0]+i[1])
        if abs(x)<=12 and abs(y)<=12:
            P.add((i,j))

# translation of elements to have start cf=0
def O(S):
    S0={((0,p[0][1]),(p[1][0]-p[0][0],p[1][1])) for p in S}
    return S0

P=O(P)

# THE STRICT STYLE

# good repetitions
R=set()
for p in P:
    # we regard unison repetition as inadmissible
    if p[0]==p[1] and p[0][1]!=0:
        R.add(p)

# parallel fifths
pf=set()
# parallel eights and unisons
pe=set()
for p in P.difference(R):
        if p[0][1]==p[1][1] and p[0][1]==7:
            pf.add(p)
        if p[0][1]==p[1][1] and p[0][1]%12==0:
            pe.add(p)

# hidden 5ths
hf=set()
# hidden 8ths and unisons
he=set()
# tritones
```

```
t=set()
# large skips (>7, not the octave)
ls=range(8,12)
sk=set()
for p in P:
    x=p[1][0]
    y=p[1][0]+p[1][1]-p[0][1]
    if p[1][1]==7 and x*y>0 and p not in pf:
        hf.add(p)
    if p[1][1]%12==0 and x*y>0 and p not in pe:
        he.add(p)
    if (abs(x)==6) or (abs(y)==6):
        t.add(p)
    if (abs(x) in ls) or (abs(y) in ls):
        sk.add(p)

# inadmissible progressions
IP=pf.union(hf,pe,he,t,sk)

# imperfect consonances by similar skips
ls=range(6,12)
skb=set()
for p in P.difference(IP):
        x=p[1][0]
        y=p[1][0]+p[1][1]-p[0][1]
        if abs(x)>2 and abs(y)>2:
            if p[1][1]%12 in {3,4,8,9} and x*y>0:
                if (abs(x) in ls) or (abs(y) in ls):
                    skb.add(p)

# hidden tritones
ht=set()
for p in P.difference(IP):
    cf=0
    dc=p[0][1]
    cf1=p[1][0]
    dc1=p[1][0]+p[1][1]
    if 6==(dc1-cf)%12 or 6==(cf1-dc)%12:
        ht.add(p)

# bad progressions
BP=skb.union(ht)

# good progressions
GP=P.difference(BP.union(IP))

print('STRICT STYLE MODULO TRANSLATION (START CF = 0)')
print(' TOTAL PROGRESSIONS:',len(P))
print('  Parallel fifths:',len(pf))
print('  Parallel eights and unisons:',len(pe))
```

```
print('  Hidden fifths:',len(hf))
print('  Hidden eights and unisons:',len(he))
print('  Tritones:',len(t))
print('  Too large skips:',len(sk))
print(' TOTAL INADMISSIBLE:',len(IP))
print('  Imp. cons. by sim. skips:',len(skb))
print('  Hidden tritones:',len(ht))
print(' TOTAL BAD:',len(BP))
print(' TOTAL GOOD:',len(GP))
```

**Code 2. Counterpoint symmetries and admitted successors**

```
# COUNTERPOINT SYMMETRIES AND ADMITTED SUCCESSORS
# Program that computes sym (k) for k in K
# and adsuc (g) for g in sym (k)

R={0,1,2,3,4,5,6,7,8,9,10,11}
Rinv={1,5,7,11}
K={0,3,4,7,8,9}
D={1,2,5,6,10,11}
b=5
a=2

alpha=0 # do alpha=1 for the first variation

# for having the gcd function
import math

# all possible values of rho
Divs= { math.gcd(i,12) for i in R}

# all posible values of the sets of the form K_i
cardK={}
for d in Divs:
    for g in range (d):
        cardK[(g,d)]=0
    for k in K:
        cardK[(k%d,d)]+=1

# the cardinality of the successors set
# for the symmetry e^v(c+d(eps))
def Sum (v,c,d):
    d=math.gcd(d,12)
    s=sum(cardK[(g,d)]*cardK[((c*g+v)%d,d)] for g in range (d))
    return d*s


# counterpoint symmetries
```

```
sym={}
# admitted successors for each counterpoint symmetry
adsuc={}
# Hichert's algorithm
for k in K:
    # maximization
    Max=0
    sym[k]=set()
    i=0
    for d in R:
        for c in Rinv:
            if (c+d*alpha)%12 in Rinv:
                for x in D:
                    v=(k-(c+d*alpha)*x)%12
                    if (b*v+a)%12==((c+d*alpha)*a+v)%12:
                        #if (b*d)%12==d%12:
                            if Sum(v,c,d)>Max:
                                Max=Sum(v,c,d)
                                sym[k]={(v,c,d)}
                            elif Sum(v,c,d)==Max:
                                sym[k].add((v,c,d))
    # admitted successors
    for g in sym[k]:
        v=g[0]
        c=g[1]
        d=g[2]
        Y=set()
        for s in R:
            for ai in K:
                if ((c+d*alpha)*ai+v+d*s)%12 in K:
                    Y.add((c*s%12,((c+d*alpha)*ai+v+d*s)%12))
                    adsuc[g]=Y

print(sym)
print(adsuc)
```

Table 1 contains the outcomes of this code.

### Code 3. Allowed and forbidden progressions

In the following codes, *one*, *two*, etc., refer to the python file names of their respective codes.

```
# ALLOWED AND FORBIDEN PROGRESSIONS
# IN A DIATONIC SCALE
from one import X, K
from two import alpha, sym, adsuc

# the set of counterpoint consonances that occur in the scale X
Cc={(x,k) for x in X for k in K if (x+k)%12 in X}
```

| $k$ | $\lvert h(K[\epsilon]) \cap K[\epsilon]\rvert$ | $h$ | Admitted successors of $k\epsilon$ |
|---|---|---|---|
| 0 | 48 | $e^{6\epsilon}(1+6\epsilon)$ | $r+\{3,9\}\epsilon$, $r$ even<br>$r+K\epsilon$, $r$ odd |
| | | $e^{6\epsilon}(7+6\epsilon)$ | $r+\{3,7,9\}\epsilon$, $r$ even<br>$r+(K\setminus\{7\})\epsilon$, $r$ odd |
| | | $e^{11\epsilon}(11+8\epsilon)$ | $\{0,3,6,9\}+\{3,4,7,8\}\epsilon$<br>$\{1,4,7,10\}+\{0,3,7,8\}\epsilon$<br>$\{2,5,8,11\}+\{0,3,4,7\}\epsilon$ |
| | | $e^{11\epsilon}(11+4\epsilon)$ | $\{0,3,6,9\}+\{3,4,7,8\}\epsilon$<br>$\{1,4,7,10\}+\{0,3,4,7\}\epsilon$<br>$\{2,5,8,11\}+\{0,3,7,8\}\epsilon$ |
| | | $e^{11\epsilon}11$ | $\mathbb{Z}_{12}+\{3,4,7,8\}\epsilon$ |
| 3 | 56 | $e^{8\epsilon}(5+8\epsilon)$ | $\{0,3,6,9\}+\{0,4,7,8\}\epsilon$<br>$\{1,4,7,10\}+(K\setminus\{7\})\epsilon$<br>$\{2,5,8,11\}+(K\setminus\{9\})\epsilon$ |
| | | $e^{8\epsilon}(5+4\epsilon)$ | $\{0,3,6,9\}+\{0,4,7,8\}\epsilon$<br>$\{1,4,7,10\}+(K\setminus\{9\})\epsilon$<br>$\{2,5,8,11\}+(K\setminus\{7\})\epsilon$ |
| 4 | 48 | $e^{6\epsilon}(1+6\epsilon)$<br>$e^{6\epsilon}(7+6\epsilon)$ | see $k=0$ |
| 7 | 60 | $e^{0}7$ | $\mathbb{Z}_{12}+(K\setminus\{7\})\epsilon$ |
| 8 | 48 | $e^{3\epsilon}7$ | $\mathbb{Z}_{12}+\{0,3,4,7\}\epsilon$ |
| | | $e^{6\epsilon}(1+6\epsilon)$<br>$e^{6\epsilon}(7+6\epsilon)$ | see $k=0$ |
| | | $e^{3\epsilon}(7+4\epsilon)$ | $\{0,3,6,9\}+\{0,3,4,7\}\epsilon$<br>$\{1,4,7,10\}+\{3,4,7,8\}\epsilon$<br>$\{2,5,8,11\}+\{0,3,7,8\}\epsilon$ |
| | | $e^{3\epsilon}(7+8\epsilon)$ | $\{0,3,6,9\}+\{0,3,4,7\}\epsilon$<br>$\{1,4,7,10\}+\{0,3,7,8\}\epsilon$<br>$\{2,5,8,11\}+\{3,4,7,8\}\epsilon$ |
| 9 | 56 | $e^{8\epsilon}(5+8\epsilon)$<br>$e^{8\epsilon}(5+4\epsilon)$ | see $k=3$ |

Table 1. Contrapuntal symmetries and admitted successors for the cantus firmus 0. We obtain the admitted successors of $z+k\epsilon$ by adding $z$ to the cantus firmus of the results.

```
# progressions in a diatonic scale (start cf=0)
P=set()
for i in Cc:
    for j in Cc:
        P.add(((0,i[1]),((j[0]-i[0])%12,j[1])))

# non-polarized progressions

NOPOL=set()
for p in P:
    if p[0][1]==p[1][1] and p[1][0] in {0,alpha*6}:
        NOPOL.add(p)
```

```
# polarized progressions
POL=P.difference(NOPOL)

# forbidden progressions
F=set()
# allowed progressions
A=set()
for p in POL:
    n=0
    for g in sym[p[0][1]]:
        if p[1] in adsuc[g]:
            n+=1
    if n==0:
        F.add(p)
    else:
        A.add(p)

print('TOTAL PROGRESSIONS: ', len(P))
print (' FORBIDDEN: ', len(F))
print (' ALLOWED: ', len(A))
print (' NON-POLARIZED: ', len(NOPOL.intersection(P)))
```

**Code 4. The reduced strict style**

```
from one import pf, pe, t, skb, ht, he, hf, sk
from one import P as Pt, IP, BP
from three import P

# reduction modulo 12
def proj(p):
    return ((0,p[0][1]%12),((p[1][0]-p[0][0])%12,p[1][1]%12))

def RO(S):
    S0={proj(p) for p in S}
    return S0

# DATA gives three integers.
# 1st number: number of inadmissible prog. projecting on p
# 2nd    "    :        "        bad            "
# 3rd    "    :        "        good           "

DATA={}
for p in P:
    DATA[p]=[0,0,0]

for p in Pt:
    if p in IP:
```

```
        DATA[proj(p)][0]+=1
    elif p in BP:
        DATA[proj(p)][1]+=1
    else:
        DATA[proj(p)][2]+=1

# REDUCED STRICT STYLE PROGRESSIONS

#  inadmissible
I=set()
#  bad
B=set()
#  good
G=set()
#  good-bad
GB=set()
#  good-good
GG=set()

for p in P:
    if DATA[p][2]>=1:
        G.add(p)
        if DATA[p][0]==0:
            if DATA[p][1]==0:
                GG.add(p)
            else:
                GB.add(p)
    else:
        if DATA[p][1]==0:
            I.add(p)
        else:
            B.add(p)

#  ambiguous
AMB=G.difference(GB,GG)

# DEDUCTIONS

#  hidden fifths from a sixth
hfs=set()
for p in P:
    x=p[1][0]
    y=p[1][0]+p[1][1]-p[0][1]
    if p[1][1]==7 and x*y>0 and p[0][1] in {8,9}:
        hfs.add(p)

print('CHARACTERIZATION␣OF␣RULES')
print('The␣other␣hid.␣par.␣without␣trit.␣that␣are␣inad.:')
hp=RO(he.union(hf))
print(hp.difference(RO(t).union (hfs)). intersection(I))
```

```
print('Proj. too large sk. that do not fall into')
print('the prev. cases and are inad.:')
# previous inadmissible cases
pc1=RO(pe).intersection(I)
pc2=RO(pf).intersection(I)
pc=pc1.union(pc2,RO(t),hfs)
print((RO(sk).difference(pc)).intersection(I))
print('The intersection of proj. too large sk.')
print('with each previous case is nonempty:')
print(' Par. eights:',len(pc1.intersection(RO(sk))))
print(' Par. fifths:',len(pc2.intersection(RO(sk))))
print(' Tritones:',len(RO(t).intersection(RO(sk))))
print(' Hid. 5ths from a 6th:',len(hfs.intersection(RO(sk))))
print('There are some bad cases:',len(B.intersection(RO(sk))))
print('There are some good cases:',len(G.intersection(RO(sk))))
sim=RO(skb).intersection(B)
print('Projected imp. cons. by sim. skips:',sim)
print('')

# REDUCED STRICT STYLE

# unrestricted validity rules (inadmissible*)
unr=(RO(pf).intersection(I)).union(RO(t))

print('REDUCED STRICT STYLE')
print(' TOTAL PROGRESSIONS:',len(P))
print(' TOTAL INADMISSIBLE:', len(I))
print(' TOTAL INADMISSIBLE*:', len(unr))
print('  Parallel fifths:', len(RO(pf).intersection(I)))
print('  Parallel unisons:', len(RO(pe).intersection(I)))
print('  Hidden fifths from a sixth:', len(hfs))
print('  Tritones:', len(RO(t)))
print(' TOTAL BAD:', len(B))
print('  Proj. imp. cons. by sim. skips:',len(sim))
print('  Hidden tritones:',len(RO(ht).intersection(B)))
print(' TOTAL GOOD:', len(G))
print(' TOTAL GOOD*:', len(G.union(I.difference(unr))))
print('  Good-good:', len(GG), GG)
print('  Good-bad:', len(GB))
print('  Ambiguous:', len(AMB))
```

**Code 5. Inadmissible, bad, and good progressions versus the model**

```
# INADMISSIBLE, GOOD, AND BAD VERSUS
# ALLOWED AND FORBIDDEN PROGRESSIONS
from three import F,A, NOPOL
from four import I,B,G,GB,GG,AMB,unr
```

```
ai=I.intersection(A)
print (' Inadmissible allowed:', len (ai))
fi=I.intersection(F)
print (' Inadmissible forbidden:', len (fi))
print (' Inadmissible non-pol.:', len (I.intersection(NOPOL)))
aiu=unr.intersection(A)
print (' Inadmissible* allowed:', len (aiu))
fiu=unr.intersection(F)
print (' Inadmissible* forbidden:', len (fiu))
print (' Bad allowed:', len (B.intersection(A)))
fb=B.intersection(F)
print (' Bad forbidden:', len (fb))
print (' Bad non-pol.:', len (B.intersection(NOPOL)))
ag=G.intersection(A)
print (' Good allowed:', len (ag))
fg=G.intersection(F)
print (' Good forbidden:', len (fg))
print (' Good non-pol.:', len (G.intersection(NOPOL)))
gu=G.union(I.difference(unr))
agu=gu.intersection(A)
print (' Good* allowed:', len (agu))
fgu=gu.intersection(F)
print (' Good* forbidden:', len (fgu))
print (' Good-bad allowed:', len ((GB.intersection(A))))
print (' Good-bad forbidden:', len (GB.intersection(F)))
print (' Good-bad non-pol.:', len (GB.intersection(NOPOL)))
agg=GG.intersection(A)
print (' Good-good allowed:', len (agg))
fgg=GG.intersection(F)
print (' Good-good forbidden:', len (fgg))
print (' Good-good non-pol.:', len (GG.intersection(NOPOL)))
print(' Ambiguous allowed:', len(AMB.intersection(A)))
print(' Ambiguous forbidden:', len(AMB.intersection(F)))
print (' Ambiguous non-pol.:', len (AMB.intersection(NOPOL)))
print('')
print('MATCHES:',len(fi)+len(ag)+len(fb))
print('MISMATCHES:',len(ai)+len(fg))
print('MATCHES*:',len(fiu)+len(agu)+len(fb))
print('MISMATCHES*:',len(aiu)+len(fgu))
print('MATCHES (ref. sem.):',len(fi)+len(agg)+len(fb))
print('MISMATCHES (ref. sem.):',len(ai)+len(fgg))
```

**Code 6. Kinds of inadmissible and bad progressions versus the model**

```
# ALLOWED AND FORBIDDEN VERSUS
# INADMISSIBLE AND BAD PROGRESSIONS

from one import pf, pe, t, skb, ht
```

```
from three import F,A
from four import I, B, RO, hfs

# intersection simplification
def j(X,Y):
    return X.intersection(Y)
def i(X,Y,Z):
    return X.intersection(Y,Z)

# inad.
print (' Par. 5ths all.:', len (i(RO(pf),I,A)))
print (' Par. 5ths forb.:', len (i(RO(pf),I,F)))
print (' Par. unisons all.:', len (i(RO(pe),I,A)))
print (' Par. unisons forb.:', len (i(RO(pe),I,F)))
print (' Hid. 5ths from a 6th all.:', len (j(hfs,A)))
print (' Hid. 5ths from a 6th forb.:', len (j(hfs,F)))
print (' Tritones all.:', len (j(RO(t),A)))
print (' Tritones forb.:', len (j(RO(t),F)))

#bad
print (' Imp. cons. by sim sk. all.:', len (i(RO(skb),B,A)))
print (' Imp. cons. by sim sk. forb.:', len (i(RO(skb),B,F)))
print (' Hid. tritones all.:', len (i(RO(ht),B,A)))
print (' Hid. tritones forb.:', len (i(RO(ht),B,F)))
```

**Code 7. The first variation**

In Code 2, we do $\alpha = 1$ in line 18. Then, we run Codes 5 and 6. They use the previous codes.

**Code 8. The final variations**

In Code 2, we comment out

```
#if (b*d)%12==d%12:
```

in line 58. Then, we run Codes 5 and 6. They use the previous codes.
